# Supplementary material for: Decoding Binding Pathways of Ligands in Prolyl Oligopeptidase
Source: arXiv:2503.15139 ancillary file (2025-03-19)
Supplement: Supplementary file 1 [file si.pdf]

# Supporting Information:

## Decoding Binding Pathways of Ligands in Prolyl Oligopeptidase

Katarzyna Walczewska-Szewc* and Jakub Rydzewski

*Institute of Physics, Faculty of Physics, Astronomy and Informatics, Nicolaus Copernicus University, Grudziadzka 5, 87-100 Toruń, Poland*

E-mail: kszewc@umk.pl

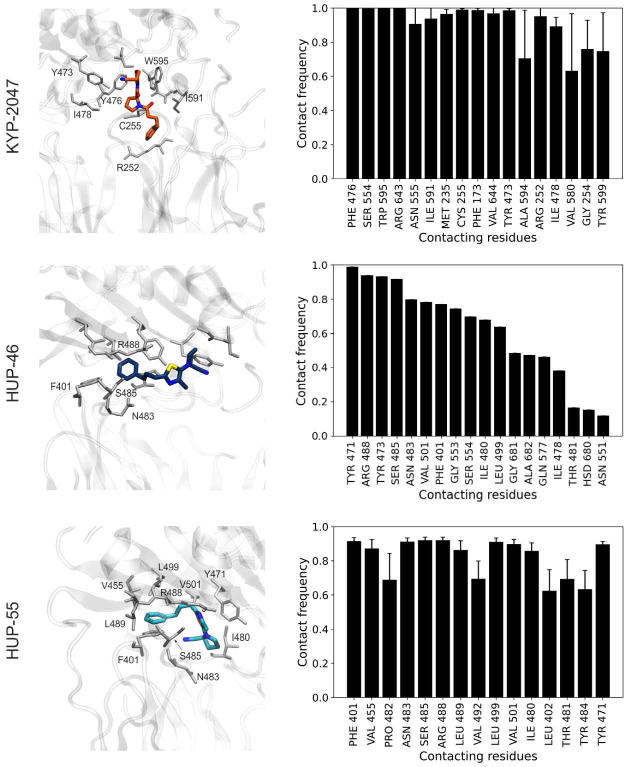


Figure S1: Visualization of ligand binding sites highlighting key protein residues involved in binding (left). The frequency of residues maintaining close contact with the ligand throughout the production run simulation (right).

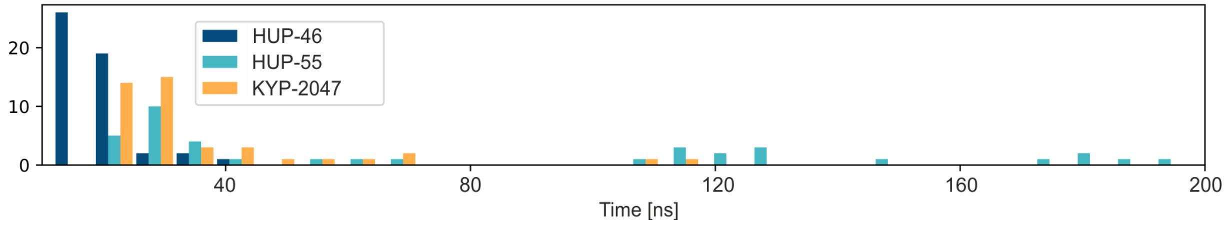


Figure S2: Distribution of times required for complete ligand unbinding events for three different ligands.

Table S1: List of the MD simulations performed in this study (cumulative time ∼17 $\mu$s).

| Protein | Ligand | Ensemble | Simulation | No. | Length [ns] |
|---|---|---|---|---|---|
| PREP | KYP-2047 | NVT | equilibration (solvent) | 1 | 0.5 |
| | | NVT | equilibration (side chains) | 3 | 1.5 |
| | | NPT | equilibration (side chains) | 1 | 1 |
| | | NPT | equilibration (unrestrained) | 1 | 50 |
| | | NPT | production MD | 5 | 500 |
| | | NPV | maze | 50 | 2-200 |
| | | NPV | umbrella sampling | 20* (×2) pathways | 10 |
| PREP | HUP-46 | NVT | equilibration (solvent) | 1 | 0.5 |
| | | NVT | equilibration (side chains) | 3 | 1.5 |
| | | NPT | equilibration (side chains) | 1 | 1 |
| | | NPT | equilibration (unrestrained) | 1 | 50 |
| | | NPT | production MD | 5 | 500 |
| | | NPV | maze | 50 | 2-200 |
| | | NPV | umbrella sampling | 20* (×2) pathways | 10 |
| PREP | HUP-55 | NVT | equilibration (solvent) | 1 | 0.5 |
| | | NVT | equilibration (side chains) | 3 | 1.5 |
| | | NPT | equilibration (side chains) | 1 | 1 |
| | | NPT | equilibration (unrestrained) | 1 | 50 |
| | | NPT | production MD | 5 | 500 |
| | | NPV | maze | 50 | 2-200 |
| | | NPV | umbrella sampling | 20* (×4) pathways | 10 |
| PREP L94C I690C | HUP-46 | NVT | equilibration (solvent) | 1 | 0.5 |
| | | NVT | equilibration (side chains) | 3 | 1.5 |
| | | NPT | equilibration (side chains) | 1 | 1 |
| | | NPT | equilibration (unrestrained) | 1 | 50 |
| | | NPT | production MD | 3 | 500 |
| | | NPV | maze | 50 | 2-200 |
| PREP T68C T686C | HUP-46 | NVT | equilibration (solvent) | 1 | 0.5 |
| | | NVT | equilibration (side chains) | 3 | 1.5 |
| | | NPT | equilibration (side chains) | 1 | 1 |
| | | NPT | equilibration (unrestrained) | 1 | 50 |
| | | NPT | production MD | 3 | 500 |
| | | NPV | maze | 50 | 2-200 |
| PREP Q397C | KYP-2047 | NVT | equilibration (solvent) | 1 | 0.5 |
| | | NVT | equilibration (side chains) | 3 | 1.5 |
| | | NPT | equilibration (side chains) | 1 | 1 |
| | | NPT | equilibration (unrestrained) | 1 | 50 |
| | | NPT | production MD | 3 | 500 |
| | | NPV | maze | 50 | 2-200 |
| PREP Q397C C255T | KYP-2047 | NVT | equilibration (solvent) | 1 | 0.5 |
| | | NVT | equilibration (side chains) | 3 | 1.5 |
| | | NPT | equilibration (side chains) | 1 | 1 |
| | | NPT | equilibration (unrestrained) | 1 | 50 |
| | | NPT | production MD | 3 | 500 |
| | | NPV | maze | 50 | 2-200 |

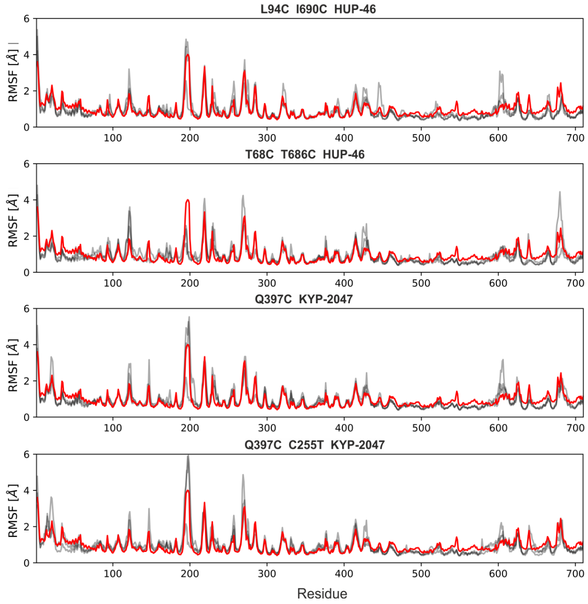


Figure S3: RMSF calculated for individual residues of the mutated (gray) and non-mutated protein (red) during production MD simulations.

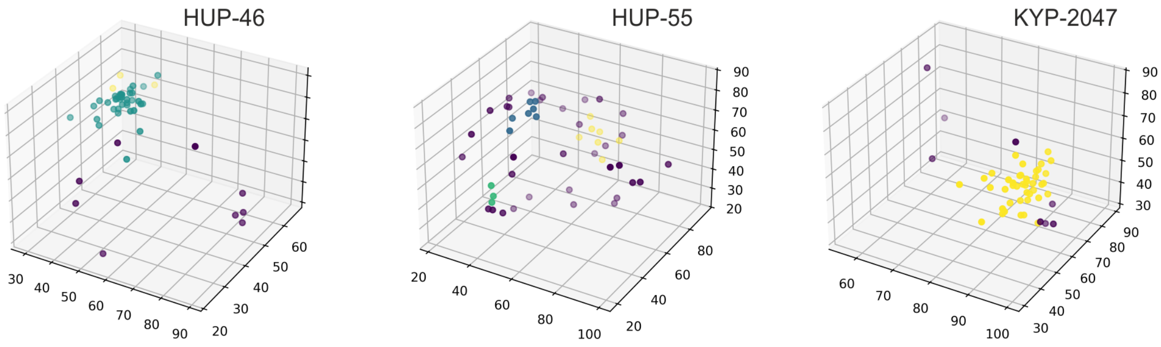


Figure S4: Final positions along the ligand exit pathway, clustered using the DBSCAN algorithm. For HUP-46 and KYP-2047, a clear preference for a specific exit region is observed (IHS for HUP-46 and the tunnel site for KYP-2047). For HUP-55, the distribution of potential exit sites is more uniform.
